# Supplementary material for: Quantum speedup for combinatorial optimization with flat energy landscapes
Source: arXiv:2306.13123 source file (2023-07-07)

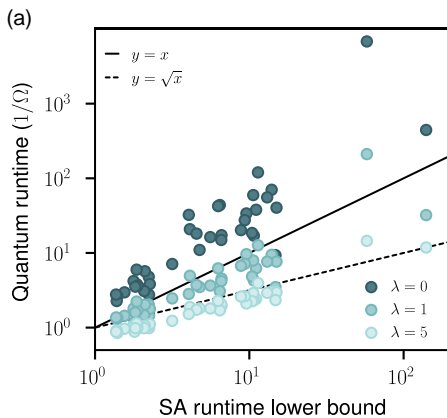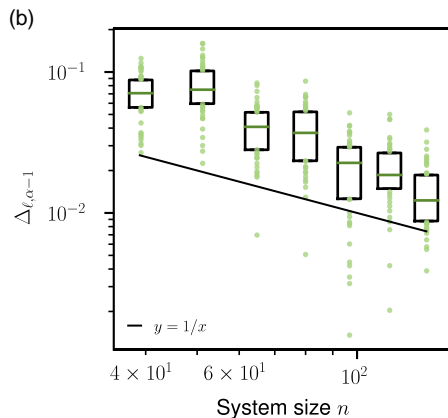

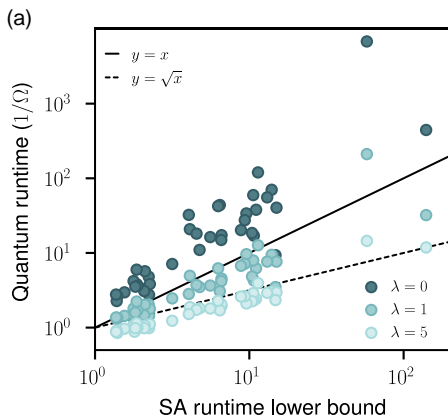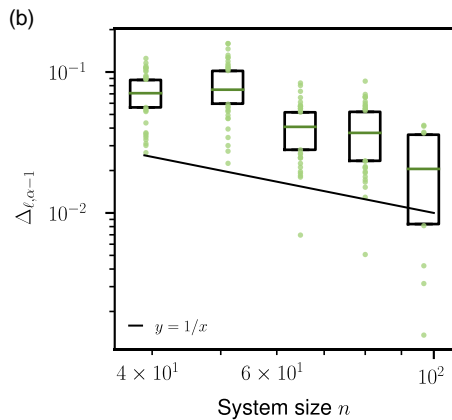

Supplement: Supplementary file 1 [file speedup_si_finite_lambda.pdf]
