# Supplementary material for: Quantum speedup for combinatorial optimization with flat energy landscapes
Source: arXiv:2306.13123 source file (2023-07-07)

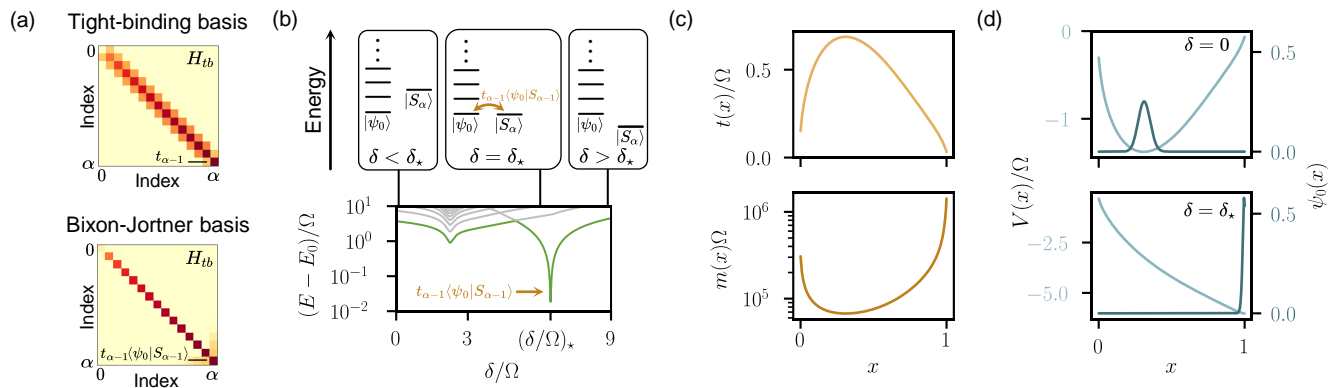

**a** Tight-binding basis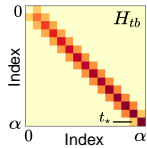

Bixon-Jortner basis

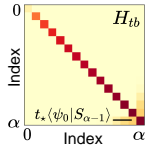**b**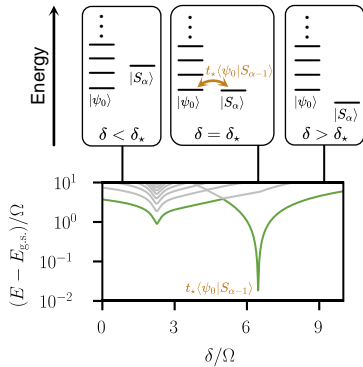**c**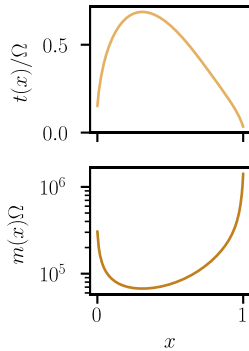**d**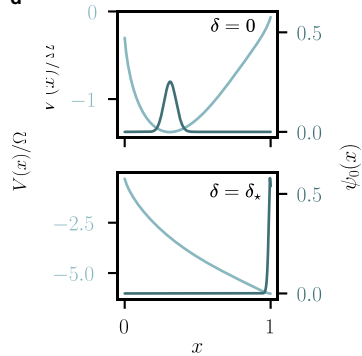

**a**

Tight-binding basis

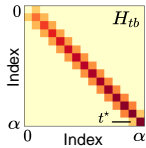

Bixon-Jortner basis

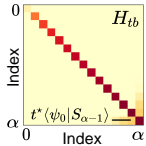**b**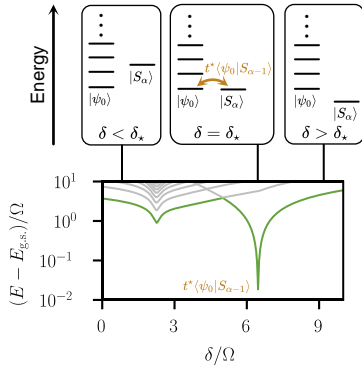**c**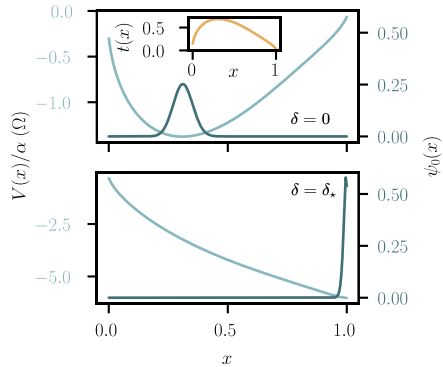

**a** Tight-binding basis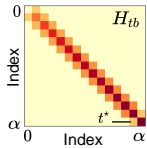

Bixon-Jortner basis

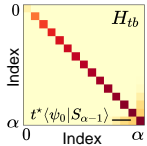**b**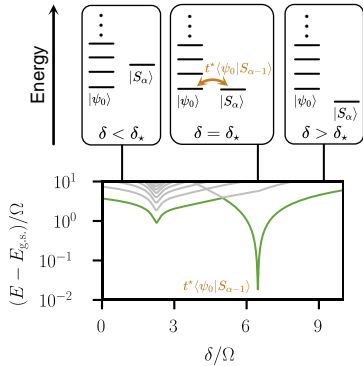**c**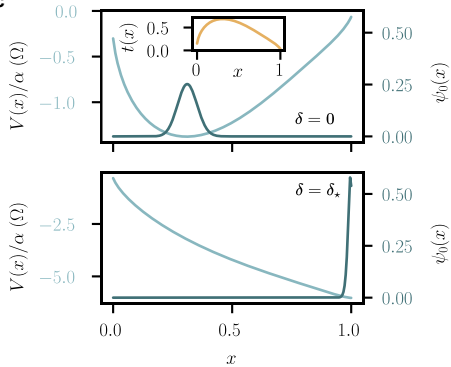

**a****Tight-binding model**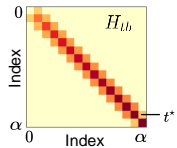**Bixon-Jortner model**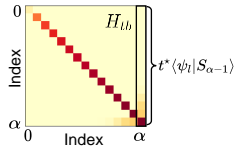**b**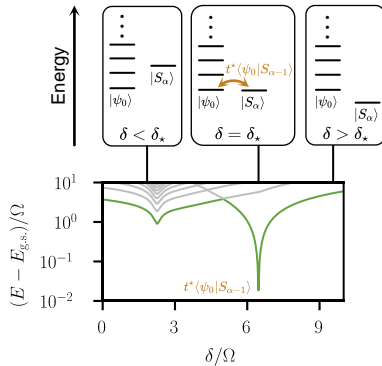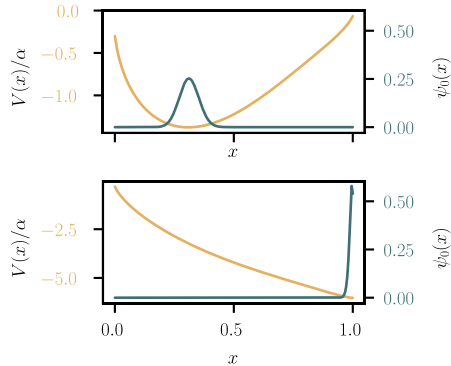

**a**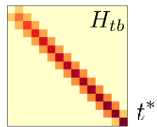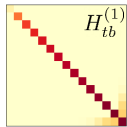**b**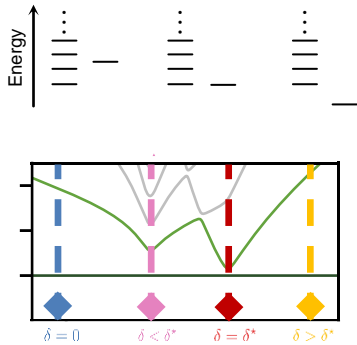

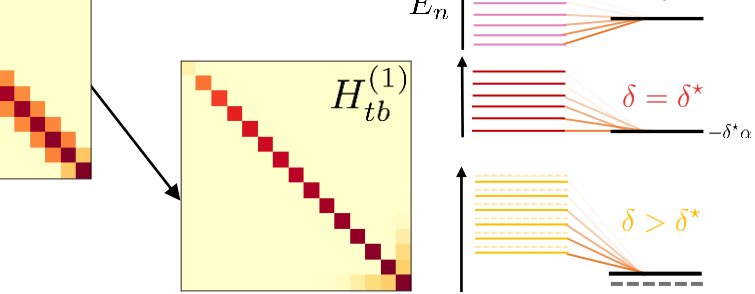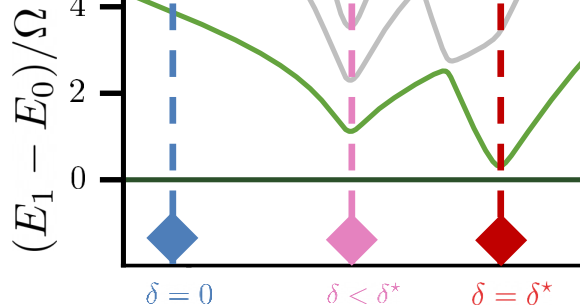

$$V(x)$$

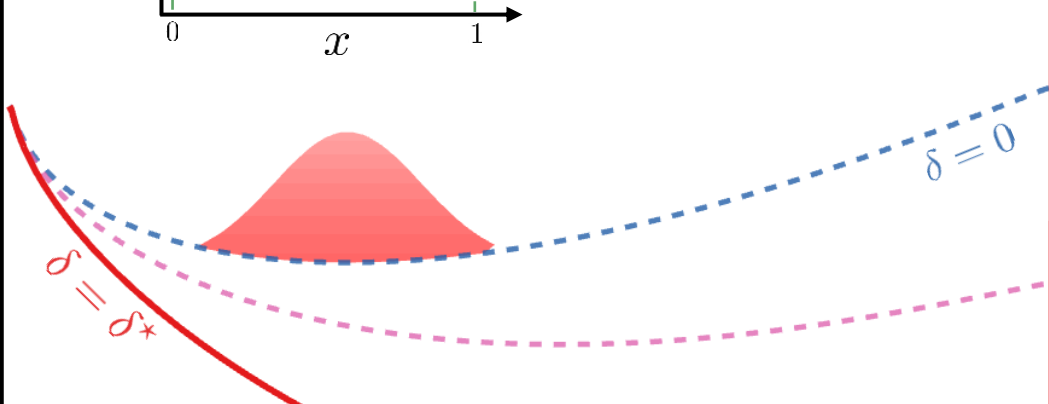



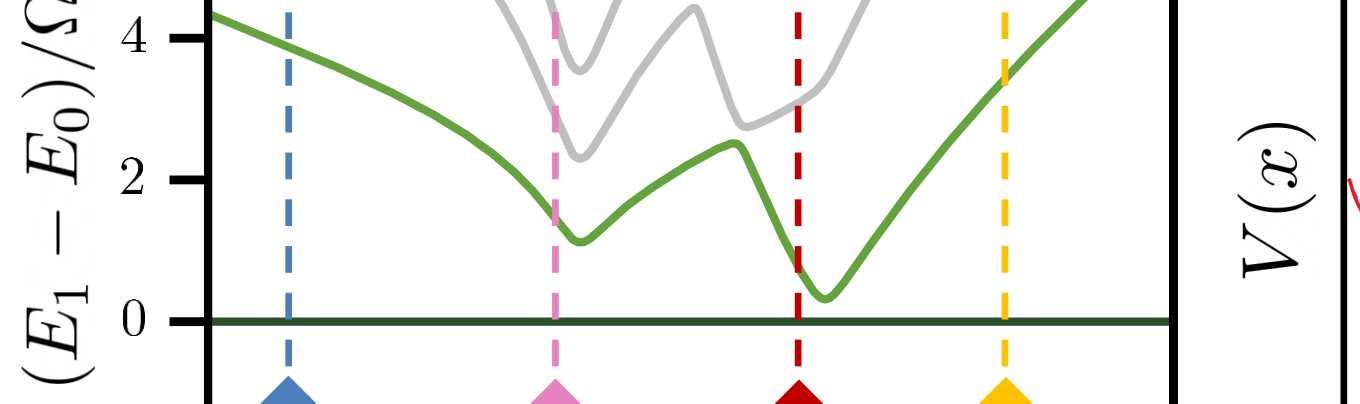

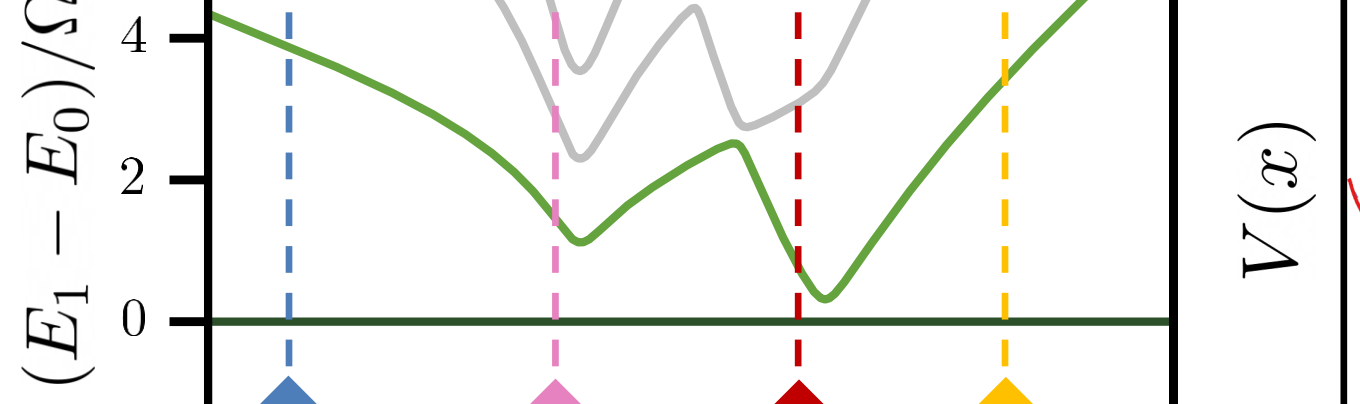

$H_{tb}$

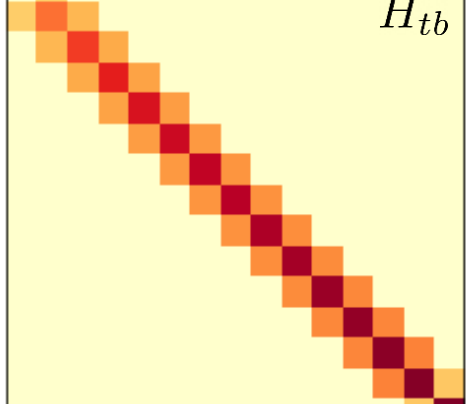

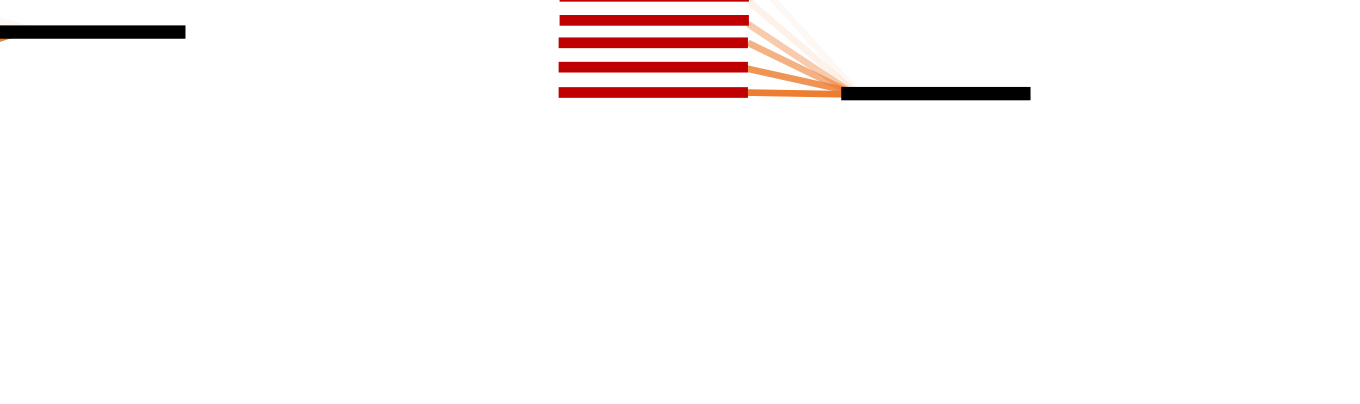



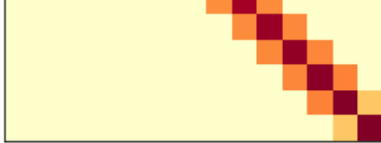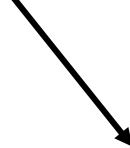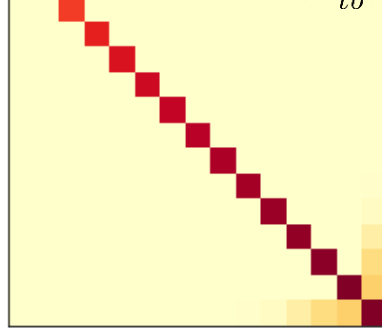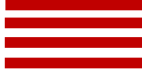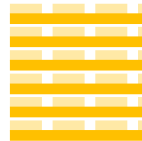

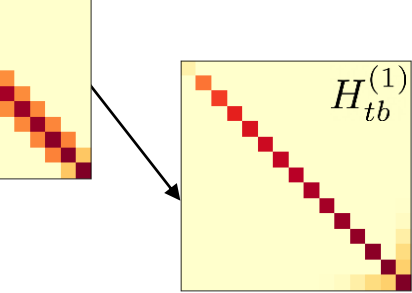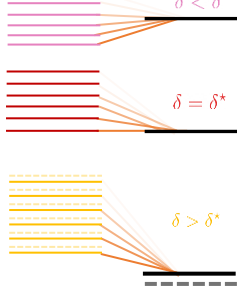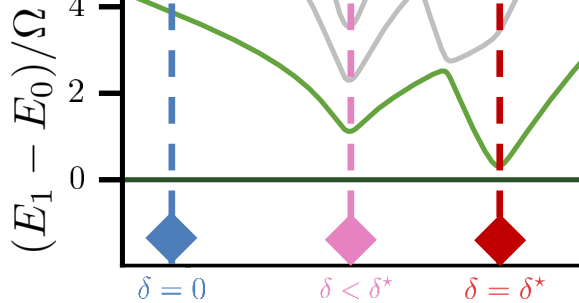

Supplement: Supplementary file 2 [file speedup_si_infinite_lambda.pdf]
