# Supplementary material for: Quantum speedup for combinatorial optimization with flat energy landscapes
Source: arXiv:2306.13123 source file (2023-07-07)

(a)

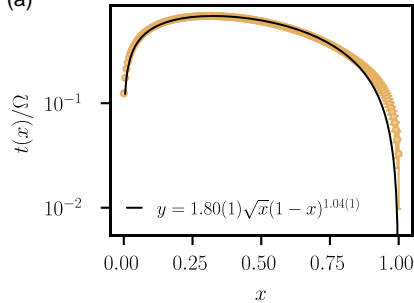

(b)

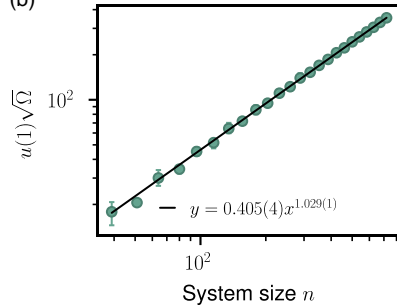

**a**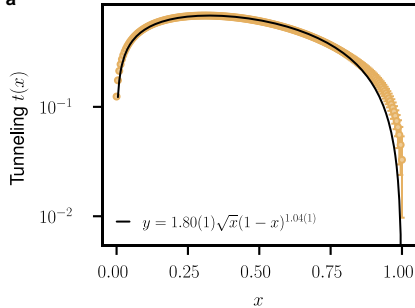**b**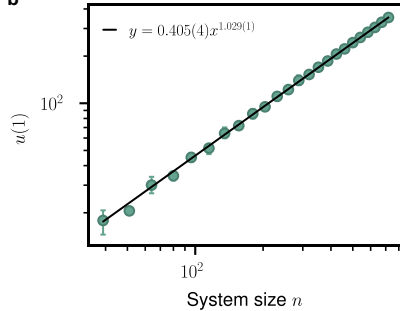

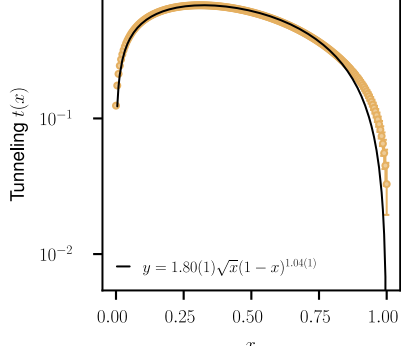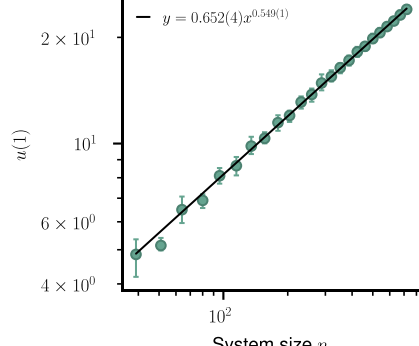

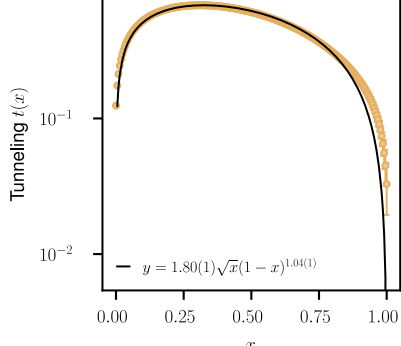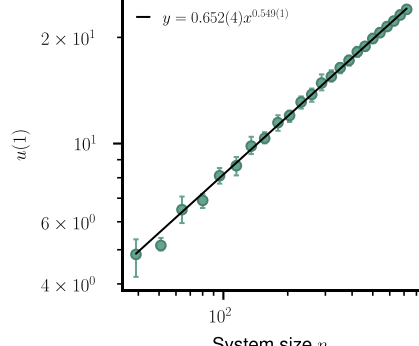

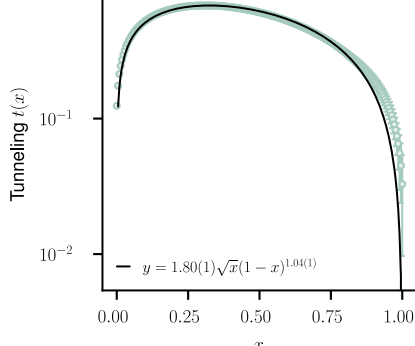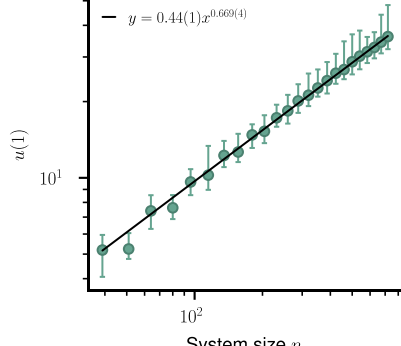

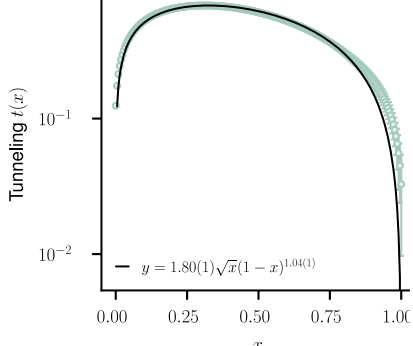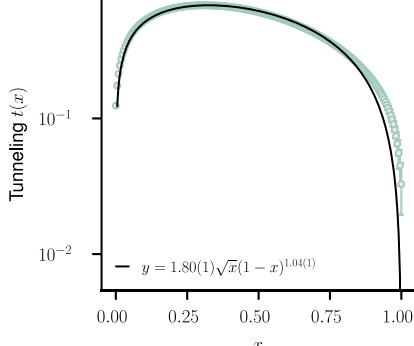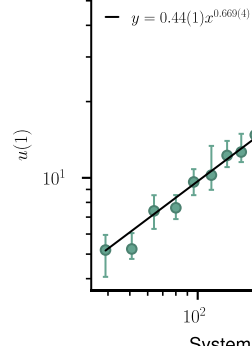

Supplement: Supplementary file 3 [file speedup_si_infinite_lambda_numerics.pdf]
