# Supplementary material for: Quantum speedup for combinatorial optimization with flat energy landscapes
Source: arXiv:2306.13123 source file (2023-07-07)

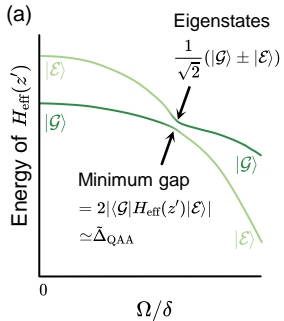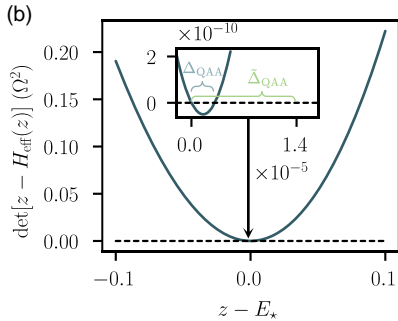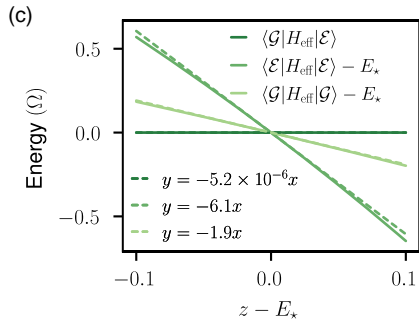

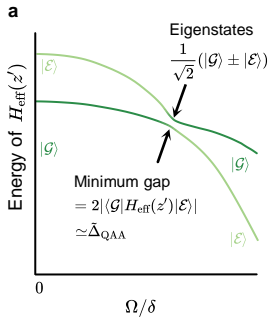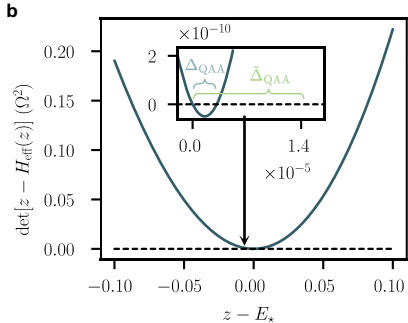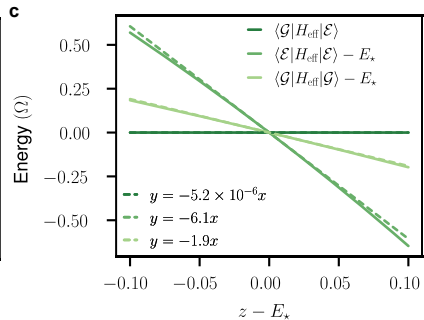

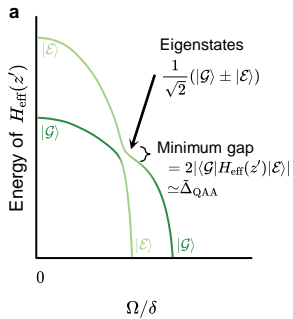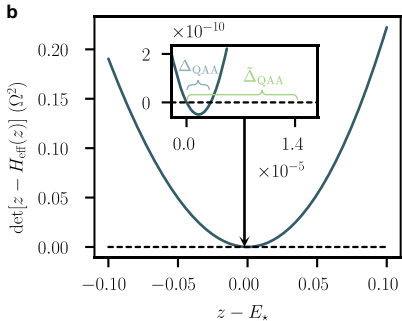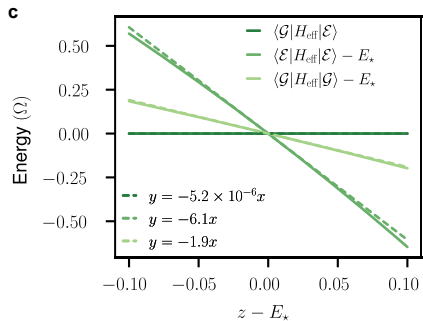

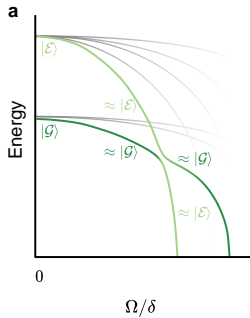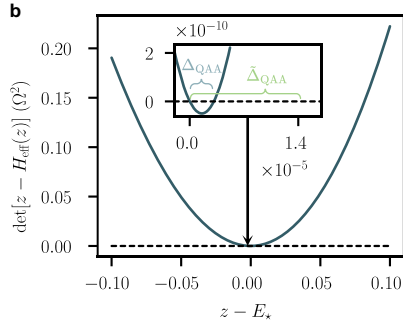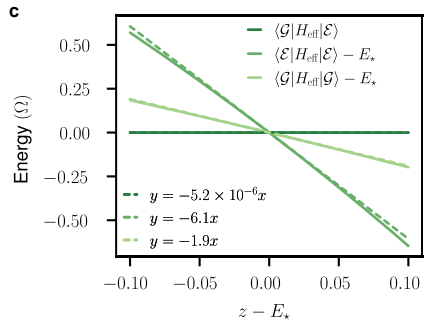

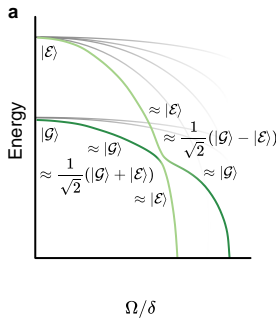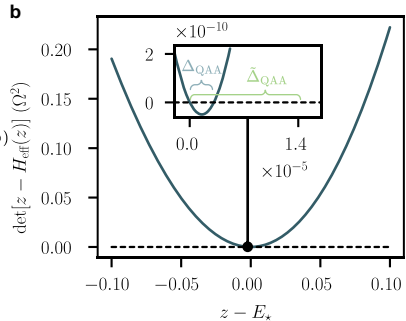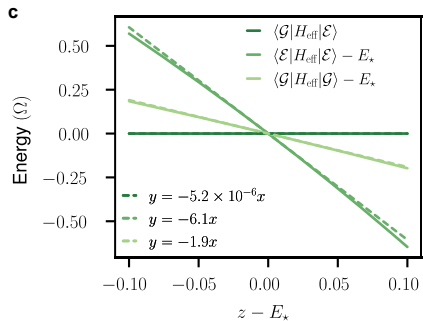

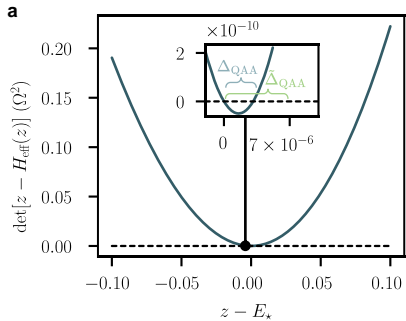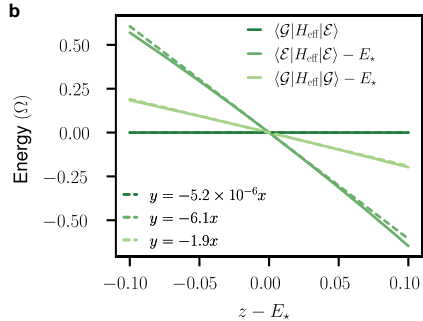

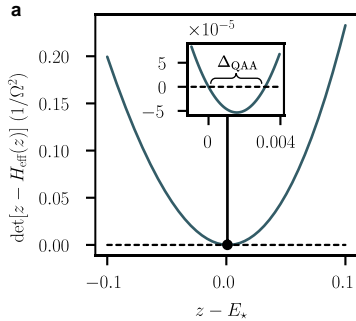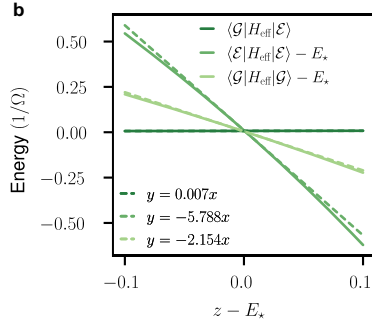

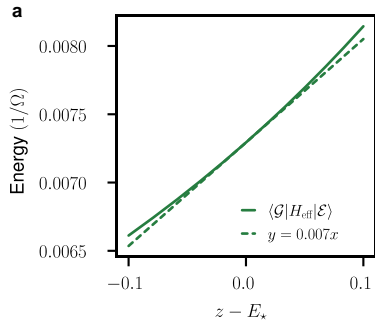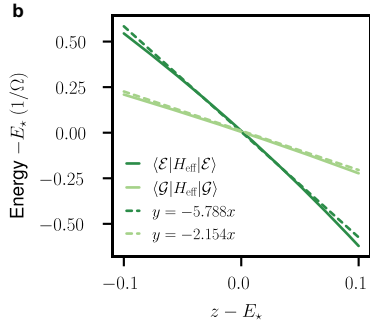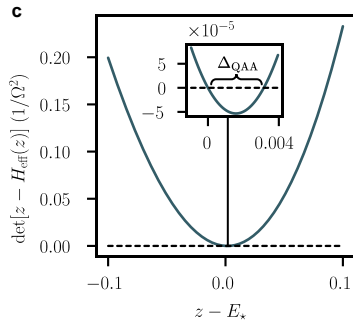

Supplement: Supplementary file 4 [file speedup_si_resolvent.pdf]
