# Supplementary material for: Quantum speedup for combinatorial optimization with flat energy landscapes
Source: arXiv:2306.13123 source file (2023-07-07)

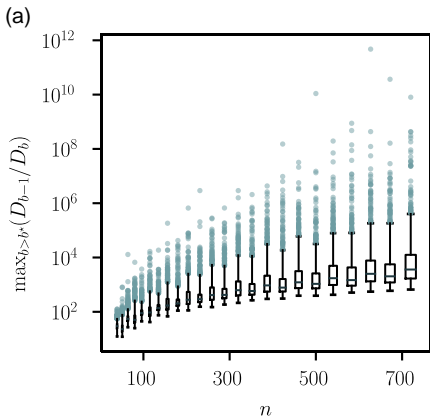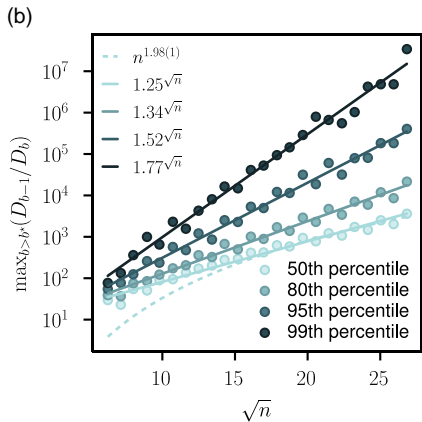

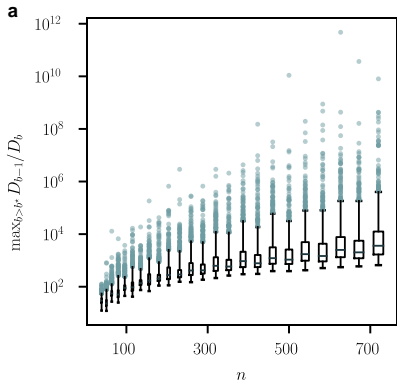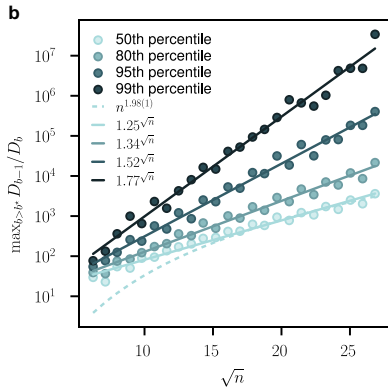

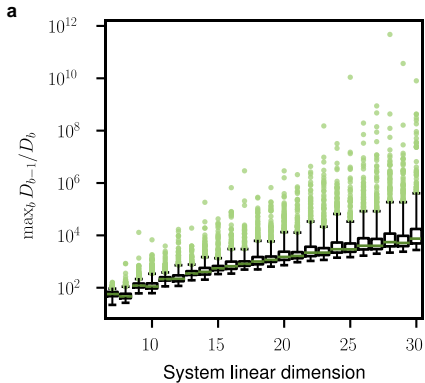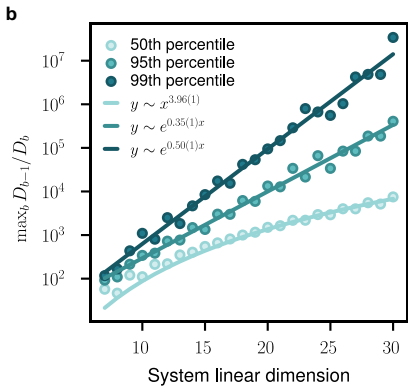

Supplement: Supplementary file 5 [file speedup_si_runtime_scaling_vs_n.pdf]
