# Supplementary material for: Quantum speedup for combinatorial optimization with flat energy landscapes
Source: arXiv:2306.13123 source file (2023-07-07)

(a)

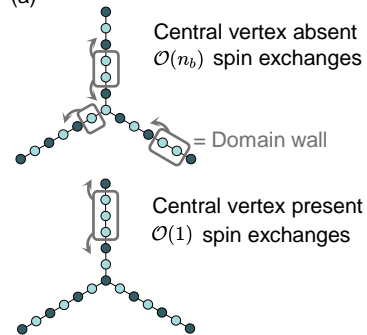

(b)

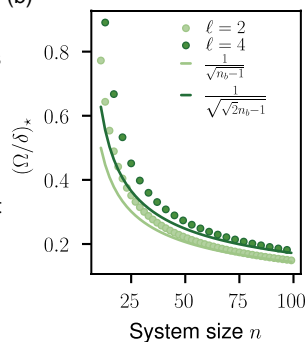

(c)

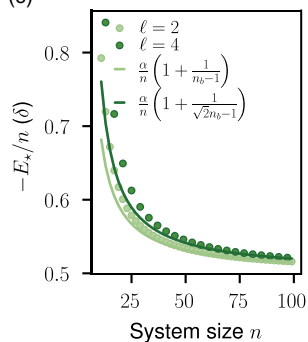

(d)

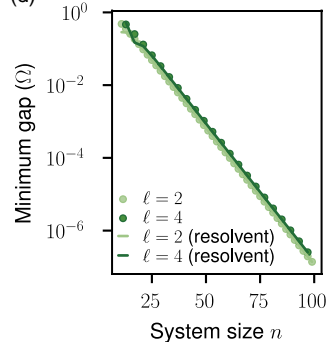

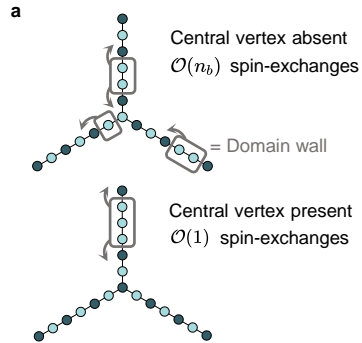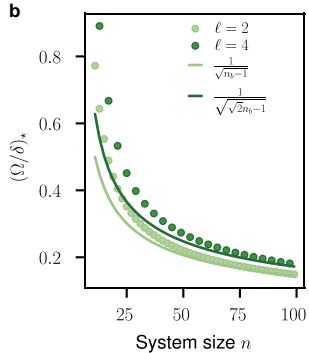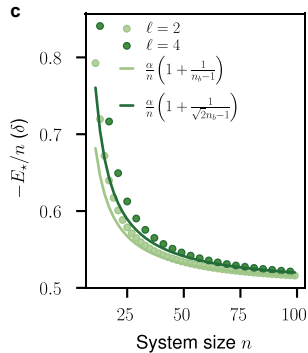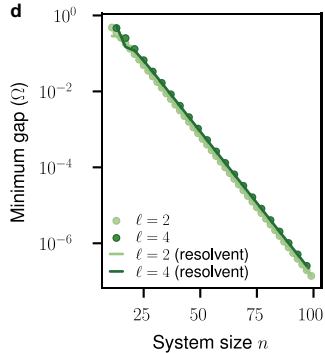

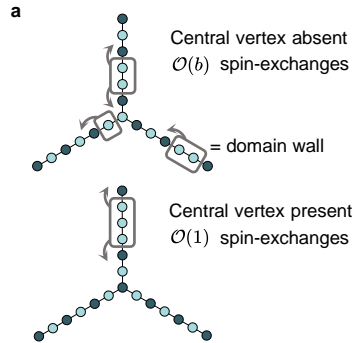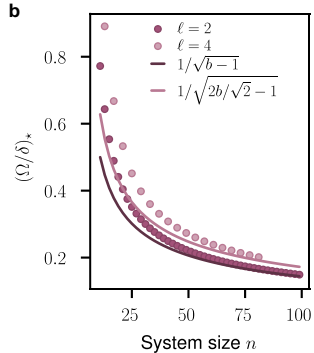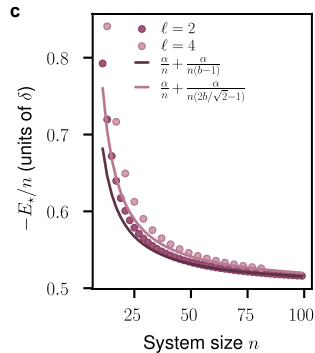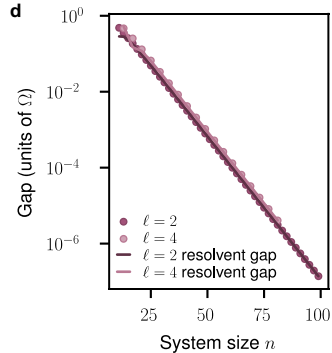

Supplement: Supplementary file 7 [file speedup_si_star.pdf]
